# Supplementary material for: The Best Instruction-Tuning Data are Those That Fit
Source: arXiv:2502.04194 source file (2026-01-11)
Supplement: Supplementary file 1 [file arr-appendix.tex]

\begin{theorem}[Ensemble Improvement with Strict Pairwise Diversity]
\label{thm:ensemble-improvement-strict}
Let $\pi^*(r \mid q_i)$ be the ground-truth distribution over responses $r$ given a query $q_i$.  Suppose $\{\pi_{\mathcal{C}}^{(m)}\}_{m=1}^M$ are $M$ component policies.  

Assume there is a constant $\gamma>1$ such that for every $r$ with $\pi^*(r\mid q_i)>0$, there is at least one policy $m$ satisfying
\begin{equation}
   \pi_{\mathcal{C}}^{(m)}(r\mid q_i)\;\ge\;\gamma \,\pi^*(r\mid q_i).
\end{equation}

Further, assume a \textbf{strict pairwise diversity} condition: for every $r$ with $\pi^*(r\mid q_i)>0$, there exist two distinct policies $m_1(r) \neq m_2(r)$ such that 
\begin{align*}
    \pi_{\mathcal{C}}^{(m_1(r))}(r \mid q_i) &> \pi_{\mathcal{C}}^{(m)}(r \mid q_i), \\
    \pi_{\mathcal{C}}^{(m_2(r))}(r \mid q_i) &> \pi_{\mathcal{C}}^{(m)}(r \mid q_i) , \\ \forall\, m \notin \{ m_1(r),\, m_2(r) \}.
\end{align*}
That is, for each such $r$, there is a \emph{pair} of policies strictly exceeding all other policies on $r.$

Then there exists a choice of nonnegative mixture weights $\{\alpha_m\}_{m=1}^M$, summing to 1, such that the mixture policy 
\[
   \pi_{\mathcal{C}}^{(\cup)}(r\mid q_i) \;=\; \sum_{m=1}^M \alpha_m\,\pi_{\mathcal{C}}^{(m)}(r\mid q_i)
\]
satisfies
\[
   D_{\mathrm{KL}}\!\bigl(\pi^*\,\big\|\,\pi_{\mathcal{C}}^{(\cup)}\bigr) \;<\;
   \min_{1\le m\le M} D_{\mathrm{KL}}\!\bigl(\pi^*\,\big\|\,\pi_{\mathcal{C}}^{(m)}\bigr).
\]
\end{theorem}

\begin{proof}
Here we provide a sketch By the definition of KL divergence, we have
\begin{equation}
\label{eq:KL-def}
\begin{split}
  &D_{\mathrm{KL}}\!\bigl(\pi^*\!\parallel\!\pi_{\mathcal{C}}^{(\cup)}\bigr)
  \;=\\&\;\sum_{r}\pi^*(r\mid q_i)\,
  \log\!\Bigl(\frac{\pi^*(r\mid q_i)}{\sum_{m=1}^M \alpha_m \,\pi_{\mathcal{C}}^{(m)}(r\mid q_i)}\Bigr).
\end{split}
\end{equation}
To ensure 
\[
   D_{\mathrm{KL}}\!\bigl(\pi^*\!\parallel\!\pi_{\mathcal{C}}^{(\cup)}\bigr)
   \;<\; D_{\mathrm{KL}}\!\bigl(\pi^*\!\parallel\!\pi_{\mathcal{C}}^{(m)}\bigr)
   \quad\forall\,m,
\]
it suffices to make the mixture probability strictly exceed each single policy's probability \emph{pointwise}, i.e.\ for every $r$ with $\pi^*(r\mid q_i)>0$,
\begin{equation}
\label{eq:ptwise-ineq}
   \sum_{m'=1}^M \alpha_{m'} \,\pi_{\mathcal{C}}^{(m')}(r\mid q_i)
   \;>\;\pi_{\mathcal{C}}^{(m)}(r\mid q_i).
\end{equation}

By strict pairwise diversity, for each $r$, there is a pair $(m_1(r), m_2(r))$ dominating all other policies on $r$.  We choose $\alpha_{m_1(r)},\alpha_{m_2(r)} > 0$ so that
\begin{align}
\begin{split}
 \alpha_{m_1(r)}\,\pi_{\mathcal{C}}^{(m_1(r))}(r\mid q_i) 
  & +  \alpha_{m_2(r)}\,\pi_{\mathcal{C}}^{(m_2(r))}(r\mid q_i)
   \; \\& >\;\max_{m}\Bigl\{\pi_{\mathcal{C}}^{(m)}(r\mid q_i)\Bigr\}.
\end{split}
\end{align}
Summing over all relevant $r$ (those with $\pi^*(r\mid q_i)>0$) to accumulate the required weights, then normalizing to ensure $\sum_{m=1}^M \alpha_m=1$, yields mixture probabilities satisfying~\eqref{eq:ptwise-ineq} for each $m$.  Hence,
\[
   D_{\mathrm{KL}}\!\bigl(\pi^*\!\parallel\!\pi_{\mathcal{C}}^{(\cup)}\bigr)
   \;<\; D_{\mathrm{KL}}\!\bigl(\pi^*\!\parallel\!\pi_{\mathcal{C}}^{(m)}\bigr)
   \quad\forall\,m,
\]
and thus
\[
   D_{\mathrm{KL}}\!\bigl(\pi^*\!\parallel\!\pi_{\mathcal{C}}^{(\cup)}\bigr)
   \;<\; \min_{1\le m\le M} D_{\mathrm{KL}}\!\bigl(\pi^*\!\parallel\!\pi_{\mathcal{C}}^{(m)}\bigr).
\]
\end{proof}

\begin{theorem}[Policy-Guided Selection Minimizes KL to $\pi_{\theta_0}$]
\label{thm:kl-minimization}
Let $\tilde{\pi}_{\mathrm{rand}}$ be any distribution supported on a random subset $\mathcal{R}_i^{(\mathrm{rand})}\subseteq \tilde{\mathcal{R}}_i$ of size $K$. Let $\hat{\pi}_{\theta_0}$ be the distribution supported on $\mathcal{R}_i^{\theta_0}$ (top-$K$ responses) and renormalized by $\pi_{\theta_0}$. Then
\[
D_{\mathrm{KL}}\Bigl(\hat{\pi}_{\theta_0}\,\Big\|\,\pi_{\theta_0}\Bigr)
\;\le\;
D_{\mathrm{KL}}\Bigl(\tilde{\pi}_{\mathrm{rand}}\,\Big\|\,\pi_{\theta_0}\Bigr).
\]
Equality holds only if $\tilde{\pi}_{\mathrm{rand}}$ places zero mass on low-$\pi_{\theta_0}$ responses and exactly matches the top-$K$ support.
\end{theorem}

\begin{proof}[Proof Sketch]
Since $\hat{\pi}_{\theta_0}$ is formed by retaining responses where $\pi_{\theta_0}(r \mid q_i)$ is highest, any alternative distribution that puts mass on responses with lower base-model probability necessarily increases the KL divergence to $\pi_{\theta_0}$. 

Concretely, KL divergence to $\pi_{\theta_0}$ is minimized by allocating probability mass \emph{proportionally} to $\pi_{\theta_0}(r \mid q_i)$ (which is exactly what $\hat{\pi}_{\theta_0}$ does). A random selection baseline $\tilde{\pi}_{\mathrm{rand}}$ can place mass on responses not favored by $\pi_{\theta_0}$, causing $\frac{\tilde{\pi}_{\mathrm{rand}}(r)}{\pi_{\theta_0}(r)}$ to become large in the KL summation. Hence 
\[
D_{\mathrm{KL}}(\tilde{\pi}_{\mathrm{rand}}\,\|\,\pi_{\theta_0}) \;>\; D_{\mathrm{KL}}(\hat{\pi}_{\theta_0}\,\|\,\pi_{\theta_0}).
\]
\end{proof}
\dylan{
Copying Hao's comments here: 
re claim 2---it is more of an intuition rather a proof. in order to prove it, you will probably make some assumptions on how the model is trained on the selected data (e.g., properly trained or achieving zero training loss). but still, i'm not sure how much significance this one has}
\dylan{
high-level thoughts on the theoretical part---i find claim 1 more interesting, but i'm not sure we are on the right path. we want to show that a student model distilled from a mixture of teachers is closer to the gold, rather than the mixture itself being close to the gold (which is what claim 1 is saying)
}
\dylan{
like we discussed earlier, i don't think it is new to distill from multiple tetacher models, but i'm not aware of any work that formally establishes the benefits of doing it from the perspective of getting closer to the gold. i haven't closely foillowed this line so you should do a careful review of the literature}
